# Supplementary material for: Matter wave lensing to picokelvin temperatures
Source: arXiv:1407.6995 ancillary file (2015-04-09)
Supplement: Supplementary file 1 [file LensingarXiv_Supplemental.pdf]

# Supplemental Materials: Matter wave lensing to picokelvin temperatures

Tim Kovachy, Jason M. Hogan, Alex Sugarbaker, Susannah M. Dickerson,
Christine A. Donnelly, Chris Overstreet, and Mark A. Kasevich
*Department of Physics, Stanford University, Stanford, California 94305*

## CONTENTS

I. Overview 1

II. Time evolution of the Wigner function in a delta-kick cooling sequence 1
A. Free space evolution 2
B. Time evolution during the delta kick 2
C. Time evolution from the lens to detection 4
D. Classical correspondence of observables calculated using the Wigner function 4
1. Expectation values immediately after the lens 5
2. Expectation values at the image plane 6
3. Results in terms of initial moments 7
E. Evaluation of position-momentum cross moments 7
F. Modified Cauchy-Schwarz inequality for symmetrized operators 9

III. Aberrations 9
A. Harmonic lens 11
B. Gaussian aberrations 12
C. High spatial frequency aberrations 13
D. Scaling of aberration contributions to cloud size with lens duration 14

IV. Point spread function 16

V. Spontaneous heating rate limit 16
A. Heating from a classicalizing modification to quantum mechanics 17
B. Analogous classical model: Fokker-Planck equation with a stochastic force 17
C. Stochastic modifications of the trajectories 18
D. Delta-kick sequence with stochastic modification 19
1. Object to lens 19
2. Lens to image 19
3. Constraining the heating rate with refocusing data 19

References 20

## I. OVERVIEW

This supplemental material presents additional details that are relevant to the main text. Section II uses a Wigner function approach to delta-kick cooling to rigorously justify the analysis of our lensing sequence in a geometric optics framework. Section III presents calculational details regarding the effect of aberrations in the lensing potential. Section IV discusses specifics of our smooth representation of the PSF. Section V provides the calculational details of the relationship between our temperature measurement and our heating rate bound.

## II. TIME EVOLUTION OF THE WIGNER FUNCTION IN A DELTA-KICK COOLING SEQUENCE

We analyze the delta-kick cooling sequence using the phase space representation of the density matrix. This allows the treatment to be valid in both the quantum and classical cases. The results we derive here are therefore applicable to the case of a pure (non-interacting) Bose-Einstein condensate and also to a classical thermal distribution of atoms.

The Wigner phase-space distribution function provides a convenient description of the dynamics because it naturally supports both the classical and quantum treatment. In the classical limit, the Wigner function time evolution equation approaches the classical Liouville equation, and so the evolution of the Wigner function in this limit is the same as the evolution of a classical thermal ensemble of particles.

### A. Free space evolution

The Wigner function for the density matrix is defined as [1]

$$W(\mathbf{r},\mathbf{p};t) = \frac{1}{(2\pi\hbar)^3}\int d^3\xi \; e^{-i\mathbf{p}\cdot\boldsymbol{\xi}/\hbar}\left\langle \mathbf{r}+\tfrac{1}{2}\boldsymbol{\xi}\right|\hat{\rho}(t)\left|\mathbf{r}-\tfrac{1}{2}\boldsymbol{\xi}\right\rangle \tag{1}$$

The time evolution of the density matrix is governed by the von Neumann equation: $i\hbar\partial_t\hat{\rho} = \left[\hat{H},\hat{\rho}\right]$, where $\hat{H} = \frac{\hat{\mathbf{p}}^2}{2m} + V(\hat{\mathbf{r}})$ is the Hamiltonian with potential energy $V(\hat{\mathbf{r}})$. For Hamiltonians that are at most second order in $\mathbf{r}$ and $\mathbf{p}$, the Wigner function evolves according to the classical Liouville equation [2]. In particular, for free space evolution $\hat{H} = \frac{\hat{\mathbf{p}}^2}{2m}$, and the quantum Liouville equation for the Wigner function is reduced to

$$\frac{\partial W(\mathbf{r},\mathbf{p};t)}{\partial t} + \frac{\mathbf{p}}{m}\cdot\boldsymbol{\nabla}_{\mathbf{r}}W(\mathbf{r},\mathbf{p};t) = 0 \qquad \text{(free space)} \tag{2}$$

The solution at time $t$ can then be expressed in terms of the Wigner function at some earlier time $t_0$ [2]:

$$W(\mathbf{r},\mathbf{p};t) = W(\mathbf{r}-\tfrac{\mathbf{p}}{m}(t-t_0),\mathbf{p};t_0) \qquad \text{(free space)} \tag{3}$$

as can be verified by inspection.

In the lens sequence, we take $t=0$ to correspond to the object plane of the lens. We assume the initial phase-space distribution function at the object plane (at $t=0$) is $W_o(\mathbf{r},\mathbf{p})$. From Eq. 3, the Wigner function after a time $t$ of free space evolution is then

$$W_{\text{free}}(\mathbf{r},\mathbf{p};t) = W_o(\mathbf{r}-\tfrac{\mathbf{p}}{m}t,\mathbf{p}). \tag{4}$$

### B. Time evolution during the delta kick

During the time that the lens is applied to the ensemble, the Hamiltonian is $\hat{H} = \frac{\hat{\mathbf{p}}^2}{2m} + V(\hat{\mathbf{r}})$, where $V(\hat{\mathbf{r}})$ is the lens potential. For an ideal lens, the lens potential should be harmonic. However, the real lens potential will contain anharmonicities that correspond to aberrations in the lens. To model these lens imperfections, we treat the lens potential as an arbitrary function $V(\hat{\mathbf{r}})$. Without loss of generality, we note that $V(\hat{\mathbf{r}})$ is roughly harmonic along the lens axes (assumed to be $x$ and $y$) plus some small aberration terms:

$$V(\hat{\mathbf{r}}) = \tfrac{1}{2}m\omega^2(\hat{x}^2+\hat{y}^2) + \delta V(\hat{\mathbf{r}}) \tag{5}$$

where $\omega$ is the nominal harmonic oscillator frequency of the lens and $\delta V(\hat{\mathbf{r}})$ is an arbitrary function that describes the aberrations.

The lens potential is assumed to turn on at time $t_o - \delta t$ and is then turned off a duration $\delta t$ later at time $t_o$. We can formally solve the von Neumann equation for the density matrix time evolution from the beginning to the end of the lens pulse:

$$\hat{\rho}(t_o) = e^{-i\hat{H}\delta t/\hbar}\hat{\rho}(t_o-\delta t)e^{i\hat{H}\delta t/\hbar} \tag{6}$$

Since the lens potential is off for times $t < t_o - \delta t$, the solution for $\hat{\rho}$ before the lens is the free space solution described in the previous section. Therefore we have as a boundary condition between the two time regions $\hat{\rho}(t_o-\delta t) = \hat{\rho}_{\text{free}}(t_o-\delta t)$, where $\hat{\rho}_{\text{free}}$ corresponds to $W_{\text{free}}$ from Eq. 4 using the definition in Eq. 1.

Next we solve for the evolution during the lens, taking advantage of the delta-kick limit. Since $\delta t$ is small, we can approximate the time evolution in Eq. 6 by splitting the Hamiltonian into a kinetic and a potential evolution operator and then evaluating the evolution from the kinetic and potential terms separately. To see this, we can formally rewrite the time evolution operator using the Zassenhaus identity

$$e^{\lambda(\hat{A}+\hat{B})} = e^{\lambda\hat{A}}e^{\lambda\hat{B}}e^{-\frac{\lambda^2}{2!}[\hat{A},\hat{B}]}e^{\frac{\lambda^3}{3!}\left(2[\hat{B},[\hat{A},\hat{B}]]+[\hat{A},[\hat{A},\hat{B}]]\right)}\cdots \tag{7}$$

for operators $\hat{A}$ and $\hat{B}$. In order to rewrite $e^{i\hat{H}\delta t/\hbar}$, we choose $\hat{A} = i\frac{\hat{\mathbf{p}}^2/2m}{\hbar\omega}$, $\hat{B} = i\frac{V(\hat{\mathbf{r}})}{\hbar\omega}$, and $\lambda = \omega\delta t$. Here we have explicitly factored out an $\omega$ from the Hamiltonian to help indicate the size of the various terms in the expansion. This choice is motivated by the fact that the scale of the Hamiltonian is set by $|H| \sim \hbar\omega$. We now use the fact that in the delta-kick limit $\omega\delta t \ll 1$, and so we have using Eq. 7

$$e^{i\left(\frac{\hat{\mathbf{p}}^2}{2m}+V(\hat{\mathbf{r}})\right)\delta t/\hbar} \approx e^{i\frac{\hat{\mathbf{p}}^2}{2m}\delta t/\hbar}\, e^{iV(\hat{\mathbf{r}})\delta t/\hbar} + \mathcal{O}(\omega\delta t)^2 \tag{8}$$

where we can neglect terms quadratic and higher in $\omega\delta t$. Combining this with Eq. 6, the Wigner function after application of the lens is

$$W(\mathbf{r},\mathbf{p};t_o) = \frac{1}{(2\pi\hbar)^3}\int d^3\xi\; e^{-i\mathbf{p}\cdot\boldsymbol{\xi}/\hbar}\left\langle \mathbf{r}+\tfrac{1}{2}\boldsymbol{\xi}\right| e^{-\frac{i}{\hbar}V(\hat{\mathbf{r}})\delta t}\left(e^{-\frac{i}{\hbar}\frac{\hat{\mathbf{p}}^2}{2m}\delta t}\hat{\rho}_{\text{free}}(t_o-\delta t)e^{\frac{i}{\hbar}\frac{\hat{\mathbf{p}}^2}{2m}\delta t}\right)e^{\frac{i}{\hbar}V(\hat{\mathbf{r}})\delta t}\left|\mathbf{r}-\tfrac{1}{2}\boldsymbol{\xi}\right\rangle \tag{9}$$

where we also have applied the previously mentioned boundary condition for $\hat{\rho}$ at time $t_o-\delta t$. The term in parenthesis simply represents additional free space time evolution by time $\delta t$, so we have

$$W(\mathbf{r},\mathbf{p};t_o) = \frac{1}{(2\pi\hbar)^3}\int d^3\xi\; e^{-i\mathbf{p}\cdot\boldsymbol{\xi}/\hbar}e^{\frac{i}{\hbar}\left(V(\mathbf{r}-\frac{1}{2}\boldsymbol{\xi})-V(\mathbf{r}+\frac{1}{2}\boldsymbol{\xi})\right)\delta t}\left\langle \mathbf{r}+\tfrac{1}{2}\boldsymbol{\xi}\right|\hat{\rho}_{\text{free}}(t_o)\left|\mathbf{r}-\tfrac{1}{2}\boldsymbol{\xi}\right\rangle \tag{10}$$

where the $V(\hat{\mathbf{r}})$ operators were applied to the adjacent position bra and ket. We now expand the potential as a Taylor series in $\xi$

$$V(\mathbf{r}\pm\tfrac{1}{2}\boldsymbol{\xi}) = \sum_{n=0}^{\infty}\frac{1}{n!}\left(\frac{\pm\boldsymbol{\xi}}{2}\cdot\boldsymbol{\nabla}_{\mathbf{r}'}\right)^n V(\mathbf{r}')\Big|_{\mathbf{r}'=\mathbf{r}} \tag{11}$$

which allows the potential terms to be combined as

$$V(\mathbf{r}-\tfrac{1}{2}\boldsymbol{\xi}) - V(\mathbf{r}+\tfrac{1}{2}\boldsymbol{\xi}) = \sum_{n=0}^{\infty}\frac{1}{n!2^{n-1}}\left(\frac{(-1)^n-1}{2}\right)(\boldsymbol{\xi}\cdot\boldsymbol{\nabla}_{\mathbf{r}'})^n V(\mathbf{r}')\Big|_{\mathbf{r}'=\mathbf{r}}. \tag{12}$$

Only the odd terms are non-zero, so we re-index the sum $n \to (2n+1)$

$$V(\mathbf{r}-\tfrac{1}{2}\boldsymbol{\xi}) - V(\mathbf{r}+\tfrac{1}{2}\boldsymbol{\xi}) = -\boldsymbol{\nabla}V(\mathbf{r})\cdot\boldsymbol{\xi} - \sum_{n=1}^{\infty}\frac{1}{(2n+1)!2^{2n}}(\boldsymbol{\xi}\cdot\boldsymbol{\nabla}_{\mathbf{r}'})^{(2n+1)}V(\mathbf{r}')\Big|_{\mathbf{r}'=\mathbf{r}} \tag{13}$$

where we have explicitly pulled the linear term out of the sum. Additionally, from the Fourier transform of Eq. 1 we have

$$\left\langle \mathbf{r}+\tfrac{1}{2}\boldsymbol{\xi}\right|\hat{\rho}_{\text{free}}(t_o)\left|\mathbf{r}-\tfrac{1}{2}\boldsymbol{\xi}\right\rangle = \int d^3p'\; e^{i\mathbf{p}'\cdot\boldsymbol{\xi}/\hbar}W_{\text{free}}(\mathbf{r},\mathbf{p}';t_o). \tag{14}$$

Combining Eq. 13 and Eq. 14 with Eq. 10 yields

$$W(\mathbf{r},\mathbf{p};t_o) = \frac{1}{(2\pi\hbar)^3}\int d^3\xi\int d^3p'\; e^{i(\mathbf{p}'-\mathbf{p}-\nabla V(\mathbf{r})\delta t)\cdot\boldsymbol{\xi}/\hbar}\; e^{-\frac{i}{\hbar}V_3(\boldsymbol{\xi})\delta t}W_{\text{free}}(\mathbf{r},\mathbf{p}';t_o) \tag{15}$$

where we have defined

$$V_3(\boldsymbol{\xi}) \equiv \sum_{n=1}^{\infty}\frac{1}{(2n+1)!2^{2n}}(\boldsymbol{\xi}\cdot\boldsymbol{\nabla}_{\mathbf{r}'})^{(2n+1)}V(\mathbf{r}')\Big|_{\mathbf{r}'=\mathbf{r}} \tag{16}$$

as a collection of terms with third order and higher odd derivatives of $V$. In the delta kick limit, we can expand the $V_3(\boldsymbol{\xi})$ exponential as

$$e^{-\frac{i}{\hbar}V_3(\boldsymbol{\xi})\delta t} \approx 1 - \tfrac{i}{\hbar\omega}V_3(\boldsymbol{\xi})\,\omega\delta t + \mathcal{O}(\omega\delta t)^2 \tag{17}$$

Next, we perform the $\xi$ integrals in Eq. 15 using the following representation of the Dirac delta function

$$\delta(\mathbf{p}) = \frac{1}{(2\pi\hbar)^3}\int d^3\xi\; e^{i\mathbf{p}\cdot\boldsymbol{\xi}/\hbar} \tag{18}$$

from which it follows that

$$\nabla_{\mathbf{p}}\delta(\mathbf{p}) = \frac{i/\hbar}{(2\pi\hbar)^3}\int d^3\xi\; \boldsymbol{\xi}\, e^{i\mathbf{p}\cdot\boldsymbol{\xi}/\hbar}. \tag{19}$$

The Fourier transforms of higher order terms in $\boldsymbol{\xi}$ then correspond to higher derivatives of delta functions. The result of the integration is

$$W(\mathbf{r},\mathbf{p};t_o) = \int d^3p' \left(\delta(\boldsymbol{\delta}\mathbf{p}) - \frac{i}{\hbar\omega}(\omega\delta t)\sum_{n=1}^{\infty}\frac{(\hbar/i)^{2n+1}}{(2n+1)!2^{2n}}\left(\boldsymbol{\nabla}_{\mathbf{p}'}\cdot\boldsymbol{\nabla}_{\mathbf{r}'}\right)^{2n+1}\delta(\boldsymbol{\delta}\mathbf{p})V(\mathbf{r}')\Big|_{\mathbf{r}'=\mathbf{r}}\right) W_{\text{free}}(\mathbf{r},\mathbf{p}';t_o) \tag{20}$$

where $\boldsymbol{\delta}\mathbf{p} \equiv \mathbf{p}' - \mathbf{p} - \nabla V\delta t$. Performing the $p'$ integrals gives the final result:

$$W(\mathbf{r},\mathbf{p};t_o) = W_{\text{free}}(\mathbf{r},\mathbf{p}-\Delta p(\mathbf{r});t_o) + \delta t\sum_{n=1}^{\infty}\frac{(-1)^n(\hbar/2)^{2n}}{(2n+1)!}\left(\boldsymbol{\nabla}_{\mathbf{p}'}\cdot\boldsymbol{\nabla}_{\mathbf{r}'}\right)^{2n+1}V(\mathbf{r}')W_{\text{free}}(\mathbf{r},\mathbf{p}';t_o)\Big|_{\mathbf{r}'=\mathbf{r},\mathbf{p}'=\mathbf{p}-\Delta p} \tag{21}$$

where the momentum impulse of the lens is defined as $\Delta p(\mathbf{r}) \equiv -\nabla V(\mathbf{r})\delta t$. The result is of the form

$$W(\mathbf{r},\mathbf{p};t_o) = W_{\text{free}}(\mathbf{r},\mathbf{p}-\Delta p(\mathbf{r});t_o) + Q \tag{22}$$

where we refer to $Q$ as the quantum term. Ignoring $Q$ for a moment, the action of the delta kick lens is to shift the momentum of the distribution by the classical momentum impulse. This is equivalent to the classical evolution of an ensemble. In this sense we may say that throughout the lens sequence the Wigner function evolves according to the classical Liouville equation. As a result, to a good approximation we may analyze the evolution of the distribution using classical physics.

The quantum term $Q$ in Eq. 22 is negligible in many relevant situations. In the delta-kick limit, a sufficiently small $(\omega\delta t)$ will ensure that $Q$ can be ignored. Additionally, since $Q$ depends only on derivatives of the potential that are third order and higher, $Q = 0$ in the case that the potential contains only terms that are second order or less in position. Even when this condition is not exactly met, we expect these higher order terms to be small compared to the second derivative terms ($\sim \omega^2$) for an approximately harmonic lens. Nevertheless, $Q$ also depends on higher order derivatives of the Wigner function, so if the initial distribution varies sufficiently rapidly with $\mathbf{p}$ then it is possible for the corrections from $Q$ to be non-negligible. To account for this possibility, we do not ignore $Q$ when using the Wigner function to calculate the experimentally observed moments of the distribution. As shown below, we find that $Q$ has no effect on these moments.

### C. Time evolution from the lens to detection

Combining Eq. 4 and Eq. 22, we can write the Wigner function immediately after the lens in terms of the initial Wigner function:

$$W(\mathbf{r},\mathbf{p};t_o) = W_o(\mathbf{r} - \tfrac{\mathbf{p}-\Delta p(\mathbf{r})}{m}t_o, \mathbf{p} - \Delta p(\mathbf{r})) \tag{23}$$

where we have ignored the quantum term $Q$. Using Eq. 3, the propagation from the lens to detection (i.e., the image plane of the lens) is given by

$$W(\mathbf{r},\mathbf{p};t_o+t_i) = W(\mathbf{r} - \tfrac{\mathbf{p}}{m}t_i, \mathbf{p}; t_o) \tag{24}$$

and so the final result for the Wigner function $W_i(\mathbf{r},\mathbf{p}) \equiv W(\mathbf{r},\mathbf{p};t_o+t_i)$ at the image plane is

$$W_i(\mathbf{r},\mathbf{p}) = W_o(\mathbf{r} - \frac{\mathbf{p}-\Delta p(\mathbf{r}-\frac{\mathbf{p}}{m}t_i)}{m}(t_o+t_i) - \frac{\Delta p(\mathbf{r}-\frac{\mathbf{p}}{m}t_i)}{m}t_i, \mathbf{p} - \Delta p(\mathbf{r}-\tfrac{\mathbf{p}}{m}t_i)) \tag{25}$$

which is the same as what is obtained using the classical Liouville equation.

### D. Classical correspondence of observables calculated using the Wigner function

Next we compute the expectation values for the position and momentum widths of the ensemble at various points in the delta-kick sequence using the Wigner function derived in the previous sections. These expectation values are our

experimental observables. In this section we show that the expectation values of the experimentally relevant moments computed using the Wigner function are all of the form

$$\langle\, g(\hat{x},\hat{p}_x)\rangle = \int d^3r \int d^3p\; g(x,p_x) W_o(\mathbf{r},\mathbf{p}) \tag{26}$$

which takes the form of a classical expectation value if $W_o(\mathbf{r},\mathbf{p})$ is identified as the classical probability distribution. Furthermore, we show explicitly that the quantum correction term $Q$ discussed in Sec. II B does not affect the moments.

The final result will depend on the initial spread of the quantum state in both $x$ and $p$, as well as cross moments between $x$ and $p$ that quantify position-momentum correlations in the cloud. However, unlike $\hat{x}$ and $\hat{p}$, we note that $\hat{x}\hat{p}$ is not a Hermitian operator, so its expectation value does not correspond to an observable. With this in mind, it is convenient to define the symmetrized operator expectation value

$$\langle A\rangle \equiv \left\langle \frac{\hat{A}+\hat{A}^\dagger}{2} \right\rangle \tag{27}$$

for a general operator $\hat{A}$ that need not be Hermitian. The symmetrized operator is guaranteed to be Hermitian, and when $\hat{A}$ itself is Hermitian we recover the normal result: $\langle A\rangle = \langle \hat{A}\rangle$. We show in Sec. II E that this symmetrized form naturally arises when computing the cross moments using the Wigner function.

### 1. *Expectation values immediately after the lens*

The first set of observables we calculate are the position and momentum widths at the time just after the lens application:

$$\Delta x_\ell^2 = \langle x_\ell^2\rangle - \langle x_\ell\rangle^2 \tag{28}$$

$$\Delta v_\ell^2 = \langle v_\ell^2\rangle - \langle v_\ell\rangle^2 \tag{29}$$

where the $\ell$ subscript indicates that the moments are evaluated at the time the lens is applied ($t = t_o$):

$$\langle x_\ell^n\rangle \equiv \langle x^n\rangle_{t=t_o} = \langle \hat{x}^n\rangle_{t=t_o} \tag{30}$$

$$\langle v_\ell^n\rangle \equiv \left\langle \left(\tfrac{p_x}{m}\right)^n\right\rangle_{t=t_o} = \langle (\hat{p}_x/m)^n\rangle_{t=t_o} \tag{31}$$

for integer $n$. The Wigner-Weyl transform of $\hat{x}$ is $x$, so we can write the $x$ moments as

$$\langle \hat{x}^n\rangle_{t=t_o} = \int d^3r \int d^3p\; x^n W(\mathbf{r},\mathbf{p};t_o) \tag{32}$$

Using Eq. 15 combined with Eq. 4,

$$\langle \hat{x}^n\rangle_{t=t_o} = \frac{1}{(2\pi\hbar)^3}\int d^3\xi \int d^3p' \int d^3r \int d^3p\; x^n e^{i(\mathbf{p}'-\mathbf{p}+\Delta p(\mathbf{r}))\cdot\boldsymbol{\xi}/\hbar}\; e^{-\frac{i}{\hbar}V_3(\boldsymbol{\xi})\delta t} W_o(\mathbf{r}-\tfrac{\mathbf{p}'}{m}t_o,\mathbf{p}') \tag{33}$$

which we note includes all the quantum terms arising from $V_3(\boldsymbol{\xi})$ discussed previously. Performing the $\mathbf{p}$ integrals results in a delta function in $\boldsymbol{\xi}$:

$$\langle \hat{x}^n\rangle_{t=t_o} = \int d^3\xi \int d^3p' \int d^3r\; x^n \delta(\boldsymbol{\xi}) e^{i(\mathbf{p}'+\Delta p(\mathbf{r}))\cdot\boldsymbol{\xi}/\hbar}\; e^{-\frac{i}{\hbar}V_3(\boldsymbol{\xi})\delta t} W_o(\mathbf{r}-\tfrac{\mathbf{p}'}{m}t_o,\mathbf{p}') \tag{34}$$

Evaluating the $\boldsymbol{\xi}$ integral eliminates the quantum terms:

$$\langle \hat{x}^n\rangle_{t=t_o} = \int d^3p' \int d^3r\; x^n W_o(\mathbf{r}-\tfrac{\mathbf{p}'}{m}t_o,\mathbf{p}'). \tag{35}$$

Finally, we perform a change of variables $\mathbf{r}\to\mathbf{r}+\frac{\mathbf{p}'}{m}t_o$ and $\mathbf{p}'\to\mathbf{p}$, yielding the final result in the form of Eq. 26:

$$\langle \hat{x}^n\rangle_{t=t_o} = \int d^3p \int d^3r\; (x+\tfrac{p_x}{m}t_o)^n W_o(\mathbf{r},\mathbf{p}). \tag{36}$$

The moments of position are therefore equivalent to the expectation values of the appropriate power of the classical position of an atom at the time of the lens.

We also calculate the momentum expectation values at the time of the lens. Once again, since the Wigner-Weyl transform of $\hat{p}_x$ is $p_x$ we can write the $p_x$ moments as

$$\langle \hat{p}_x^n \rangle_{t=t_o} = \int d^3r \int d^3p \; p_x^n W(\mathbf{r}, \mathbf{p}; t_o) \tag{37}$$

Proceeding along the same lines as for the position moments,

$$\langle \hat{p}_x^n \rangle_{t=t_o} = \frac{1}{(2\pi\hbar)^3} \int d^3\xi \int d^3p' \int d^3r \int d^3p \; p_x^n e^{i(\mathbf{p}' - \mathbf{p} + \Delta p(\mathbf{r}))\cdot \boldsymbol{\xi}/\hbar} \; e^{-\frac{i}{\hbar} V_3(\boldsymbol{\xi})\delta t} W_o(\mathbf{r} - \tfrac{\mathbf{p}'}{m} t_o, \mathbf{p}') \tag{38}$$

$$= \int d^3\xi \int d^3p' \int d^3r \; \frac{\hbar^n}{(-i)^n} \frac{\partial^n \delta(\boldsymbol{\xi})}{\partial \xi_x^n} e^{i(\mathbf{p}' + \Delta p(\mathbf{r}))\cdot \boldsymbol{\xi}/\hbar} \; e^{-\frac{i}{\hbar} V_3(\boldsymbol{\xi})\delta t} W_o(\mathbf{r} - \tfrac{\mathbf{p}'}{m} t_o, \mathbf{p}') \tag{39}$$

where the $p$ integral results in the $n$th derivative of the Dirac delta function with respect to $\xi_x$. Next, for the $\boldsymbol{\xi}$ integral we have that

$$\int d^3\xi \; \frac{\partial^n \delta(\boldsymbol{\xi})}{\partial \xi_x^n} h(\boldsymbol{\xi}) = (-1)^n \frac{\partial^n h(\boldsymbol{\xi})}{\partial \xi_x^n}\Big|_{\boldsymbol{\xi}=0} \tag{40}$$

for any function $h(\boldsymbol{\xi})$. For the case at hand, $h(\boldsymbol{\xi}) = e^{\frac{i}{\hbar}(\mathbf{p}' + \Delta p(\mathbf{r}))\cdot \boldsymbol{\xi} - V_3(\boldsymbol{\xi})\delta t)}$. As a result of the $\boldsymbol{\xi}$-dependence of $V_3$, the lowest two derivative have a particularly simple form:

$$\frac{\partial h(\boldsymbol{\xi})}{\partial \xi_x}\Big|_{\boldsymbol{\xi}=0} = \frac{i}{\hbar}(p_x' + \Delta p_x(\mathbf{r})) \tag{41}$$

$$\frac{\partial^2 h(\boldsymbol{\xi})}{\partial \xi_x^2}\Big|_{\boldsymbol{\xi}=0} = \left(\frac{i}{\hbar}\right)^2 (p_x' + \Delta p_x(\mathbf{r}))^2 \tag{42}$$

Note that higher derivatives will give quantum corrections arising from $V_3$, but for $n \leq 2$ these do not contribute. Thus after computing the $\boldsymbol{\xi}$ integrals we have for $n \leq 2$

$$\langle \hat{p}_x^n \rangle_{t=t_o} = \int d^3p' \int d^3r \; \frac{\hbar^n}{(-i)^n} (-1)^n \left(\frac{i}{\hbar}\right)^n (p_x' + \Delta p_x(\mathbf{r}))^n W_o(\mathbf{r} - \tfrac{\mathbf{p}'}{m} t_o, \mathbf{p}') \qquad (n \leq 2) \tag{43}$$

$$= \int d^3p' \int d^3r \; (p_x' + \Delta p_x(\mathbf{r}))^n W_o(\mathbf{r} - \tfrac{\mathbf{p}'}{m} t_o, \mathbf{p}') \tag{44}$$

As before, we perform a change of variables $\mathbf{r} \to \mathbf{r} + \frac{\mathbf{p}'}{m} t_o$ and $\mathbf{p}' \to \mathbf{p}$ yielding the final result:

$$\langle \hat{p}_x^n \rangle_{t=t_o} = \int d^3p \int d^3r \; (p_x + \Delta p_x(\mathbf{r} + \tfrac{\mathbf{p}}{m} t_o))^n W_o(\mathbf{r}, \mathbf{p}) \qquad (n \leq 2). \tag{45}$$

Just like the moments of position, the moments of momentum are therefore equivalent to the expectation values of the appropriate power of the classical momentum of an atom immediately after the lens, where the second term ($\Delta p_x$) accounts for the classical momentum kick imparted by the lens.

### 2. *Expectation values at the image plane*

Next we calculate the width of the ensemble at the image plane:

$$\langle \Delta x_i^2 \rangle = \langle x_i^2 \rangle - \langle x_i \rangle^2 \tag{46}$$

This corresponds to the experimentally observed cloud width at detection. Here the $i$ subscript indicates that the moments are evaluated at the image plane of the lens ($t = t_o + t_i$):

$$\langle x_i^n \rangle \equiv \langle x^n \rangle_{t=t_o+t_i} = \langle \hat{x}^n \rangle_{t=t_o+t_i} \tag{47}$$

Using the Wigner function at the image plane, the $x$ moments can be written

$$\langle \hat{x}^n \rangle_{t=t_o+t_i} = \int d^3r \int d^3p \; x^n W(\mathbf{r},\mathbf{p};t_o+t_i) \tag{48}$$

$$= \int d^3r \int d^3p \; x^n W(\mathbf{r}-\tfrac{\mathbf{p}}{m}t_i,\mathbf{p};t_o) \tag{49}$$

$$= \int d^3r \int d^3p \; (x+\tfrac{p_x}{m}t_i)^n W(\mathbf{r},\mathbf{p};t_o) \tag{50}$$

where we took advantage of Eq. 24 in the second line and did a change of variable in the third line. Using Eq. 15,

$$\langle \hat{x}^n \rangle_{t=t_o+t_i} = \frac{1}{(2\pi\hbar)^3}\int d^3\xi \int d^3p' \int d^3r \int d^3p \; (x+\tfrac{p_x}{m}t_i)^n \, e^{i(\mathbf{p}'-\mathbf{p}+\Delta p(\mathbf{r}))\cdot\boldsymbol{\xi}/\hbar} \; e^{-\frac{i}{\hbar}V_3(\boldsymbol{\xi})\delta t} W_o(\mathbf{r}-\tfrac{\mathbf{p}'}{m}t_o,\mathbf{p}') \tag{51}$$

It is now convenient to use the change of variables $\mathbf{r}'' \equiv \mathbf{r}$ and $\mathbf{p}'' \equiv \frac{m}{t_i}\mathbf{r}+\mathbf{p}$ so that

$$\langle \hat{x}^n \rangle_{t=t_o+t_i} = \frac{1}{(2\pi\hbar)^3}\int d^3\xi \int d^3p' \int d^3r'' \int d^3p'' \; (\tfrac{p''_x}{m}t_i)^n \, e^{i(\mathbf{p}'-\mathbf{p}''+\frac{m}{t_i}\mathbf{r}''+\Delta p(\mathbf{r}''))\cdot\boldsymbol{\xi}/\hbar} \; e^{-\frac{i}{\hbar}V_3(\boldsymbol{\xi})\delta t} W_o(\mathbf{r}''-\tfrac{\mathbf{p}'}{m}t_o,\mathbf{p}') \tag{52}$$

Next we formally define a shifted momentum impulse $\overline{\Delta p}(\mathbf{r}'') \equiv \Delta p(\mathbf{r}'') + \frac{m}{t_i}\mathbf{r}''$. With this identification, we can use the fact that Eq. 52 is of the same form as Eq. 38 with $\Delta p \to \overline{\Delta p}$. Therefore we have

$$\langle \hat{x}^n \rangle_{t=t_o+t_i} = \left(\tfrac{t_i}{m}\right)^n \langle \hat{p}^n \rangle_{t=t_o}\big|_{\Delta p\to\overline{\Delta p}} \tag{53}$$

$$= \left(\tfrac{t_i}{m}\right)^n \int d^3p \int d^3r \; (p_x + \Delta p_x(\mathbf{r}+\tfrac{\mathbf{p}}{m}t_o) + \tfrac{m}{t_i}(x+\tfrac{p_x}{m}t_o))^n W_o(\mathbf{r},\mathbf{p}) \qquad (n \le 2). \tag{54}$$

where we used the result from Eq. 45. Thus we arrive at the final result

$$\langle \hat{x}^n \rangle_{t=t_o+t_i} = \int d^3p \int d^3r \; (x + \tfrac{p_x}{m}(t_o+t_i) + \tfrac{1}{m}\Delta p_x(\mathbf{r}+\tfrac{\mathbf{p}}{m}t_o)\, t_i)^n W_o(\mathbf{r},\mathbf{p}) \qquad (n \le 2). \tag{55}$$

which is of the form of the expectation value of moments of the classical position at detection.

### 3. *Results in terms of initial moments*

It is possible to write the results for each of the measured moments explicitly in terms of expectation values of the initial moments of the distribution:

$$\Delta x_o^2 = \langle x_o^2 \rangle - \langle x_o \rangle^2 \tag{56}$$

$$\Delta v_o^2 = \langle v_o^2 \rangle - \langle v_o \rangle^2 \tag{57}$$

$$\langle \Delta x_o \Delta v_o \rangle = \langle x_o v_o \rangle - \langle x_o \rangle \langle v_o \rangle \tag{58}$$

where the cross moments are defined using Eq. 27. This is desirable because the initial moments are the experimentally defined quantities. The conversion requires performing an inverse Wigner-Weyl transform on the arguments of the integral in Eq. 55 (and equivalent for the other moments). This process will result in expectation values of symmetrized operators. Since we only consider first and second order moments, the only terms that we must consider are of the form $x^2$, $p_x^2$, $\Delta p_x^2(\mathbf{r}+\frac{\mathbf{p}}{m}t_o)$, $xp$, $p_x\Delta p_x(\mathbf{r}+\frac{\mathbf{p}}{m}t_o)$, and $x\Delta p_x(\mathbf{r}+\frac{\mathbf{p}}{m}t_o)$. The inverse Wigner-Weyl transforms of $x^2$ and $p_x^2$ are trivial, and the transform of $xp$ is $(\hat{x}\hat{p}+\hat{p}\hat{x})/2$, but the transforms of $p_x\Delta p_x$, $x\Delta p_x$, and $\Delta p_x^2$ are less obvious. In the following section we prove that the latter three terms can be written as symmetrized expectation values, even for arbitrary functions $\Delta p_x(\mathbf{r})$.

## E. Evaluation of position-momentum cross moments

In calculating the effect of the lens on the atom distribution, it will be necessary to convert terms of the form

$$C_f \equiv \int d^3x d^3p \; p_x f\left(\mathbf{r}+\frac{\mathbf{p}}{m}t_o\right) W_o(\mathbf{r},\mathbf{p}) \tag{59}$$

into expectation values of appropriate operators. We assume that $f$ is real-valued and that it can be Taylor expanded in its arguments. Using Eq. 4 and a change of variables, we can alternatively write

$$C_f = \int d^3x d^3p \; p_x f\left(\mathbf{r}\right) W_{\text{free}}(\mathbf{r},\mathbf{p};t_o) = \int d^3x d^3p \; p_x \left(\sum_{i,j,k} f_{i,j,k} x^i y^j z^k\right) W_{\text{free}}(\mathbf{r},\mathbf{p};t_o) \tag{60}$$

$$= \sum_{i,j,k} f_{i,j,k} \int d^3x d^3p \; p_x x^i y^j z^k W_{\text{free}}(\mathbf{r},\mathbf{p};t_o) \tag{61}$$

where $f_{i,j,k}$ are the appropriate Taylor series coefficients for $f\left(\mathbf{r}\right)$. Since the Wigner-Weyl transform of the symmetrized operator $(\hat{p}_x \hat{x}^i \hat{y}^j \hat{z}^k + \hat{x}^i \hat{y}^j \hat{z}^k \hat{p}_x)/2$ gives $p_x x^i y^j z^k$, we can write this series as

$$C_f = \sum_{i,j,k} f_{i,j,k} \left\langle \frac{\hat{p}_x \hat{x}^i \hat{y}^j \hat{z}^k + \hat{x}^i \hat{y}^j \hat{z}^k \hat{p}_x}{2} \right\rangle_{t=t_o} \tag{62}$$

$$= \left\langle \frac{\hat{p}_x \left(\sum_{i,j,k} f_{i,j,k} \hat{x}^i \hat{y}^j \hat{z}^k\right) + \left(\sum_{i,j,k} f_{i,j,k} \hat{x}^i \hat{y}^j \hat{z}^k\right) \hat{p}_x}{2} \right\rangle_{t=t_o} \tag{63}$$

$$= \left\langle \frac{\hat{p}_x f\left(\hat{\mathbf{r}}\right) + f\left(\hat{\mathbf{r}}\right) \hat{p}_x}{2} \right\rangle_{t=t_o} . \tag{64}$$

We will now express $C_f$ as an expectation value evaluated at $t=0$. In the Heisenberg picture, we can write Eq. 64 as

$$C_f = \left\langle \frac{\hat{p}_x(t_o) f\left(\hat{\mathbf{r}}(t_o)\right) + f\left(\hat{\mathbf{r}}(t_o)\right) \hat{p}_x(t_o)}{2} \right\rangle_{t=0} \tag{65}$$

where the subscript indicates that the expectation value is evaluated using the state at $t=0$. The operators at $t=t_o$ are related to the operators at $t=0$ by

$$\hat{\mathbf{r}}(t_o) = \hat{\mathbf{r}}(0) + \frac{\hat{\mathbf{p}}(0)}{m} t_o \tag{66}$$

$$\hat{\mathbf{p}}(t_o) = \hat{\mathbf{p}}(0), \tag{67}$$

so

$$C_f = \left\langle \frac{\hat{p}_x(0) f\left(\hat{\mathbf{r}}(0) + \frac{\hat{\mathbf{p}}(0)}{m} t_o\right) + f\left(\hat{\mathbf{r}}(0) + \frac{\hat{\mathbf{p}}(0)}{m} t_o\right) \hat{p}_x(0)}{2} \right\rangle_{t=0} . \tag{68}$$

In Schrödinger picture notation, this is simply

$$C_f = \left\langle \frac{\hat{p}_x f\left(\hat{\mathbf{r}} + \frac{\hat{\mathbf{p}}}{m} t_o\right) + f\left(\hat{\mathbf{r}} + \frac{\hat{\mathbf{p}}}{m} t_o\right) \hat{p}_x}{2} \right\rangle_{t=0} \equiv \left\langle p_x f\left(\mathbf{r} + \frac{\mathbf{p}}{m} t_o\right)\right\rangle, \tag{69}$$

using the symmetrized operator expectation value notation defined in Eq. 27 for the final equality. A similar argument demonstrates that the $x\Delta p_x$ term can be written as

$$\left\langle \frac{\hat{x} \Delta p_x\left(\hat{\mathbf{r}} + \frac{\hat{\mathbf{p}}}{m} t_o\right) + \Delta p_x\left(\hat{\mathbf{r}} + \frac{\hat{\mathbf{p}}}{m} t_o\right) \hat{x}}{2} \right\rangle_{t=0} \equiv \left\langle x \Delta p_x\left(\mathbf{r} + \frac{\mathbf{p}}{m} t_o\right)\right\rangle \tag{70}$$

and that the $\Delta p_x^2$ term can be written as

$$\left\langle \Delta p_x^2 (\hat{\mathbf{r}} + \tfrac{\hat{\mathbf{p}}}{m} t_o)\right\rangle_{t=0} \equiv \left\langle \Delta p_x^2 (\mathbf{r} + \tfrac{\mathbf{p}}{m} t_o)\right\rangle . \tag{71}$$

### F. Modified Cauchy-Schwarz inequality for symmetrized operators

We now derive a modified Cauchy-Schwarz inequality for symmetrized operators that is needed to prove our claims in the following section. This inequality states that for Hermitian operators $\hat{A}$ and $\hat{B}$,

$$\left\langle A^2\right\rangle\left\langle B^2\right\rangle - \left\langle AB\right\rangle^2 \equiv \left\langle \hat{A}^2\right\rangle\left\langle \hat{B}^2\right\rangle - \left\langle \frac{\hat{A}\hat{B}+\hat{B}\hat{A}}{2}\right\rangle^2 \geq 0, \tag{72}$$

where once again we use the symmetrized operator expectation value notation. The lefthand side of this inequality can be written as a sum of two terms which are independently $\geq 0$:

$$\left\langle A^2\right\rangle\left\langle B^2\right\rangle - \left\langle AB\right\rangle^2 = \Gamma_1 + \Gamma_2 \tag{73}$$

where

$$\Gamma_1 = \left\langle \hat{A}^2\right\rangle\left\langle \hat{B}^2\right\rangle - \left\langle \hat{A}\hat{B}\right\rangle\left\langle \hat{B}\hat{A}\right\rangle = \left\langle \hat{A}^2\right\rangle\left\langle \hat{B}^2\right\rangle - \left|\left\langle \hat{A}\hat{B}\right\rangle\right|^2 \tag{74}$$

$$\Gamma_2 = -\frac{1}{4}\left[\left\langle \hat{A}\hat{B}\right\rangle^2 + \left\langle \hat{B}\hat{A}\right\rangle^2 - 2\left\langle \hat{A}\hat{B}\right\rangle\left\langle \hat{B}\hat{A}\right\rangle\right] = -\frac{1}{4}\left[\left\langle \hat{A}\hat{B}\right\rangle - \left\langle \hat{B}\hat{A}\right\rangle\right]^2 = -\frac{1}{4}\left\langle\left[\hat{A},\hat{B}\right]\right\rangle^2. \tag{75}$$

The fact that $\Gamma_1 \geq 0$ follows directly from the standard Cauchy-Schwarz inequality for Hermitian operators. Because $\hat{A}$ and $\hat{B}$ are Hermitian, the expectation value of their commutator is purely imaginary, giving us $\Gamma_2 \geq 0$.

## III. ABERRATIONS

Here we analyze the effect that aberrations in the lens potential have on the ability to collimate and refocus atoms in a delta kick cooling procedure. The lens potential can deviate from the ideal harmonic form for a variety of reasons. For the optical dipole lens like the one used in this work, these include deviations due to the Gaussian profile of the laser beam as well as higher spatial frequency intensity variations arising from imperfections in the delivery optics. Other types of lens potentials (e.g., magnetic fields) can suffer from analogous aberrations. In the main text we use a lens based on a TOP trap where aberrations result from the fact that the magnetic trap is effectively harmonic only over a limited spatial extent.

To model the lens aberrations, we consider an arbitrary position-dependent lens force $F(x)$ acting on the atoms during the brief lens operation. In the harmonic limit, this force reduces to the simple case discussed in the paper, $F(x) \to -m\omega^2 x$, but for now we allow $F(x)$ to remain completely general. For this analysis we consider the delta-kick (thin lens) limit discussed in Sec. II, where we may treat the action of the lens as delivering a position-dependent momentum impulse $F(x)\delta t$. This approximation holds as long as the atom does not move much during the lens pulse so that the force is roughly constant.

As established in Sec. II, we can calculate the experimentally relevant moments in terms of symmetrized operator expectation values (discussed in Sec. II D) by considering the evolution of classical trajectories in phase space. Immediately after the lens is applied, a given classical trajectory with initial $x$-position $x_o$ and initial velocity $v_o$ in the $x$-direction has the form

$$x_\ell = x_o + v_o t_o \tag{76}$$

$$v_\ell = v_o + a(x_\ell, y_\ell)\delta t, \tag{77}$$

where we have defined the lens induced acceleration in the $x$-direction as $a(x,y) = F(x,y)/m$ and where $y$ is the orthogonal transverse direction. As discussed above, when calculating moments, we integrate over the $y$-dependence of the trajectories. To emphasize this, we suppress the $y$-dependence of $a$ in subsequent equations.

At the image plane, the trajectory has final position

$$x_i = x_o + v_o(t_o + t_i) + a(x_\ell)t_i\delta t. \tag{78}$$

We are interested in evaluating the collimation performance of the lens – that is, how cold are the atoms immediately after applying the lens. Computing expectation values using Eq. 77, the second moment of the velocity after the lens is

$$\left\langle v_\ell^2\right\rangle = \left\langle v_o^2\right\rangle + 2\delta t\left\langle v_o a\right\rangle + \delta t^2\left\langle a^2\right\rangle \tag{79}$$

and the square of the mean velocity is

$$\langle v_\ell \rangle^2 = \langle v_o \rangle^2 + 2 \langle v_o \rangle \langle a \rangle \delta t + \langle a \rangle^2 \delta t^2 \tag{80}$$

where $a \equiv a(x_\ell) = a(x_o + v_o t_o)$. The velocity variance after the lens is $\Delta v_\ell^2 \equiv \langle v_\ell^2 \rangle - \langle v_\ell \rangle^2$. Choosing the lens duration $\delta t_c$ to minimize the velocity variance, we obtain

$$\delta t_c = -\frac{\langle \Delta v_o \Delta a \rangle}{\Delta a^2}, \tag{81}$$

and the minimum (collimated) velocity variance after the lens is given by

$$\Delta v_\ell^2 = \frac{\Delta v_o^2 \Delta a^2 - \langle \Delta v_o \Delta a \rangle^2}{\Delta a^2} \tag{82}$$

where $\langle \Delta x \Delta y \rangle \equiv \langle (x - \langle x \rangle)(y - \langle y \rangle) \rangle = \langle xy \rangle - \langle x \rangle \langle y \rangle$ and $\Delta a^2 \equiv \langle a^2 \rangle - \langle a \rangle^2$. This velocity width corresponds to the coldest temperatures that can be produced by the lens.

In the main text, we characterize the performance of the lens by observing the RMS size of the ensemble at detection. From Eq. 78, the second moment of the position at detection is

$$\langle x_i^2 \rangle = \langle (x_o + v_o(t_o + t_i))^2 \rangle + 2 \langle x_o a \rangle t_i \delta t + 2 \langle v_o a \rangle (t_o + t_i) t_i \delta t + \langle a^2 \rangle t_i^2 \delta t^2 \tag{83}$$

and the square of the mean position is

$$\langle x_i \rangle^2 = \langle x_o \rangle^2 + 2 \langle x_o \rangle \langle v_o \rangle (t_o + t_i) + \langle v_o \rangle^2 (t_o + t_i)^2 + 2 (\langle x_o \rangle + \langle v_o \rangle (t_o + t_i)) \langle a \rangle t_i \delta t + \langle a \rangle^2 t_i^2 \delta t^2. \tag{84}$$

The ensemble width at detection is $\Delta x_i^2 \equiv \langle x_i^2 \rangle - \langle x_i \rangle^2$ and may be written in the form that appears in Eq. 2 in the main text:

$$\Delta x_i^2 = (\Delta x_i)^2_{\min} + \Delta a^2 t_i^2 (\delta t - \delta t_{\min})^2 \tag{85}$$

where $(\Delta x_i)_{\min}$ is the mimimum width, $\Delta a^2 = \Delta F^2/m$, and $\delta t_{\min}$ is the lens duration that minimizes Eq. 83. We find that

$$\delta t_{\min} = -\frac{\langle \Delta x_\ell \Delta a \rangle}{\Delta a^2} \left( \frac{1}{t_i} + \frac{1}{t_o} \left( 1 - \frac{\langle \Delta x_o \Delta a \rangle}{\langle \Delta x_\ell \Delta a \rangle} \right) \right) \tag{86}$$

and

$$\begin{aligned} (\Delta x_i)^2_{\min} = t_i^2 & \left( \frac{\Delta v_o^2 \Delta a^2 - \langle \Delta v_o \Delta a \rangle^2}{\Delta a^2} \right) \\ & + \left( 1 + 2\frac{t_i}{t_o} \right) \left( \frac{\Delta x_\ell^2 \Delta a^2 - \langle \Delta x_\ell \Delta a \rangle^2}{\Delta a^2} \right) - 2\frac{t_i}{t_o} \left( \frac{\langle \Delta x_o \Delta x_\ell \rangle \Delta a^2 - \langle \Delta x_\ell \Delta a \rangle \langle \Delta x_o \Delta a \rangle}{\Delta a^2} \right). \end{aligned} \tag{87}$$

In the main text we define the measured ensemble RMS velocity as $(\Delta v_\ell)^2_{\text{bound}} \equiv (\Delta x_i)^2_{\min}/t_i^2$. Combining Eqs. 82 and 87, we arrive at Eq. 1 from the main text, namely

$$(\Delta v_\ell)^2_{\text{bound}} = \Delta v_\ell^2 + \delta A \tag{88}$$

where we define the aberration during refocusing $\delta A$ as

$$\delta A \equiv \frac{1}{t_i^2} \left[ \left( 1 + 2\frac{t_i}{t_o} \right) \left( \frac{\Delta x_\ell^2 \Delta a^2 - \langle \Delta x_\ell \Delta a \rangle^2}{\Delta a^2} \right) - 2\frac{t_i}{t_o} \left( \frac{\langle \Delta x_o \Delta x_\ell \rangle \Delta a^2 - \langle \Delta x_\ell \Delta a \rangle \langle \Delta x_o \Delta a \rangle}{\Delta a^2} \right) \right]. \tag{89}$$

It is important to note that $\Delta v_\ell$ in Eq. 88 includes effects from aberrations during collimation and is therefore the physical minimum RMS velocity that can be reached with this particular lens. We can therefore use $(\Delta v_\ell)_{\text{bound}}$ to set an upper bound on the coldest possible ensemble that can be produced with this lens, accounting for aberration in both $\Delta v_\ell$ and the observed $(\Delta x_i)_{\min}$.

In order for the experimentally inferred $(\Delta v_\ell)_{\rm bound}$ to be an upper bound for the minimum RMS velocity $\Delta v_\ell$, we must have $\delta A \geq 0$. Using the fact that $x_\ell = x_o + v_o t_o$, we may rewrite $\delta A$ as

$$\delta A = \frac{1}{t_i^2}\left(1+\frac{t_i}{t_o}\right)\left(\frac{\Delta x_\ell^2 \Delta a^2 - \langle \Delta x_\ell \Delta a\rangle^2}{\Delta a^2}\right) + \frac{t_o}{t_i}\left(\frac{\Delta v_o^2 \Delta a^2 - \langle \Delta v_o \Delta a\rangle^2}{\Delta a^2}\right) - \frac{1}{t_i t_o}\left(\frac{\Delta x_o^2 \Delta a^2 - \langle \Delta x_o \Delta a\rangle^2}{\Delta a^2}\right). \quad (90)$$

The first two terms in this expression are non-negative by the Cauchy-Schwarz inequality, and the magnitude of the third term is bounded by the Cauchy-Schwarz inequality (here, we are using the Cauchy-Schwarz inequality for symmetrized operators derived in Sec. II F). Allowing the third term to be as negative as possible, and taking the first two terms to be zero, we arrive at a lower bound on $\delta A$:

$$\delta A \geq -\frac{\Delta x_o^2}{t_i t_o}. \quad (91)$$

Thus, even though $\delta A$ is not strictly positive for arbitrary potentials and intial phase space distributions, $\delta A$ can provide only a small negative contribution to $(\Delta v_\ell)_{\rm bound}$ even in the worst case. For our parameters, this worst-case contribution is still smaller than the stated uncertainty in the temperature bound reported in the main text and can be neglected.

A potentially stronger lower bound on $\delta A$ can be obtained by writing the lens acceleration $a(x_\ell)$ as the sum of harmonic and aberration terms:

$$a(x_\ell) = -\omega^2 x_\ell + \delta a(x_\ell). \quad (92)$$

Here the linear effect of the aberrations has been incorporated into the definition of $\omega$, so

$$\omega^2 = -\frac{\langle \Delta x_\ell \Delta a\rangle}{\Delta x_\ell^2} \quad (93)$$

and $\langle \Delta x_\ell \Delta \delta a\rangle = 0$. Substituting $a = -\omega^2 x_\ell + \delta a$ into Eq. 90, we obtain

$$\delta A = \frac{\Delta x_\ell^2}{t_i^2 \Delta a^2}\left(\left(1+\frac{t_i}{t_o}+\frac{\Delta v_o^2 t_o^2 - \Delta x_o^2}{\Delta x_\ell^2}\right)\Delta\delta a^2 - 2\frac{t_i}{t_o}\omega^2\langle \Delta x_o \Delta \delta a\rangle\right). \quad (94)$$

From this expression, we see that if the lens is harmonic (i.e. if $\delta a = 0$), then $\delta A = 0$. In addition, we have $\delta A \geq 0$ as long as

$$\Delta\delta a^2 \geq \frac{2\frac{t_i}{t_o}}{1+\frac{t_i}{t_o}+\frac{\Delta v_o^2 t_o^2 - \Delta x_o^2}{\Delta x_\ell^2}}\,\omega^2\langle \Delta x_o \Delta\delta a\rangle. \quad (95)$$

In the worst case, $\langle \Delta x_o \Delta \delta a\rangle = \sqrt{\Delta x_o^2 \Delta \delta a^2} = \Delta x_o \Delta\delta a$ by the Cauchy-Schwarz inequality, and $\delta A \geq 0$ if

$$\Delta\delta a \geq \frac{2\frac{t_i}{t_o}}{1+\frac{t_i}{t_o}+\frac{\Delta v_o^2 t_o^2 - \Delta x_o^2}{\Delta x_\ell^2}}\,\omega^2\Delta x_o \sim \omega^2 \Delta x_o. \quad (96)$$

Thus, lens aberrations are guaranteed to contribute positively to the image size as long as the aberration-induced acceleration is larger than the scale set by $\omega^2 \Delta x_o$. We also show explicitly that $\delta A > 0$ for a lensing potential with Gaussian aberrations (see section III B), which are the dominant source of aberrations in our experiment. Thus $\delta A \geq 0$ for the results stated in this paper, and $(\Delta v_\ell)_{\rm bound}$ is an upper bound on the minimum velocity width $\Delta v_\ell$.

### A. Harmonic lens

With no aberrations, $a(x) = -\omega^2 x$. Then from Eq. 81, the lensing time required to collimate the cloud is

$$\delta t_c = \frac{1}{\omega^2}\frac{\langle \Delta v_o \Delta x_o\rangle + t_o \Delta v_o^2}{\Delta x_\ell^2}. \quad (97)$$

If there are no correlations between $x_o$ and $v_o$ in the initial cloud, we can rewrite the expression for $\delta t_c$ to obtain

$$\delta t_c = \frac{1}{\omega^2}\frac{t_o \Delta v_o^2}{\Delta x_\ell^2} = \frac{1}{\omega^2 t_o}\frac{\Delta x_\ell^2 - \Delta x_o^2}{\Delta x_\ell^2} = \frac{1}{\omega^2 t_o}(1-\gamma^2) \quad (98)$$

which implies a focal time of

$$f_c \equiv \frac{1}{\omega^2 \delta t_c} = \frac{t_o}{1-\gamma^2}. \tag{99}$$

Here $\gamma \equiv \frac{\Delta x_o}{\Delta x_\ell}$ is the ratio of the initial cloud width to the cloud width at the lens. The minimum achievable velocity width is calculated from Eq. 82 to be

$$\Delta v_\ell^2 = \Delta v_o^2 \gamma^2 - \frac{\langle \Delta v_o \Delta x_o \rangle^2}{\Delta x_\ell^2} \tag{100}$$

In the absence of correlations between $x_o$ and $v_o$, the lens reduces the effective temperature of the cloud by a factor of

$$\eta_c \equiv \frac{\Delta v_\ell^2}{\Delta v_o^2} = \gamma^2 \tag{101}$$

at collimation.

From Eq. 85, the RMS position width at the imaging time is

$$\Delta x_i^2 = (\Delta x_i)^2_{\min} + \omega^4 \Delta x_\ell^2 t_i^2 \left(\delta t - \delta t_{\min}\right)^2. \tag{102}$$

The lens time required to achieve the minimum RMS position width is given by Eq. 86,

$$\delta t_{\min} = \frac{1}{\omega^2}\left(\frac{1}{t_i} + \frac{1}{t_o}\left(1 - \frac{\langle \Delta x_o \Delta x_\ell \rangle}{\Delta x_\ell^2}\right)\right) = \frac{1}{\omega^2}\left(\frac{1}{t_i} + \frac{1}{t_o}(1-\gamma^2) - \frac{\langle \Delta x_o \Delta v_o \rangle}{\Delta x_\ell^2}\right) \tag{103}$$

and the minimum RMS position width is given by Eq. 87,

$$(\Delta x_i)^2_{\min} = \frac{t_i^2}{\Delta x_\ell^2}\left(\Delta v_o^2 \Delta x_o^2 - \langle \Delta v_o \Delta x_o \rangle^2\right) = t_i^2 \Delta v_o^2 \gamma^2 - \frac{t_i^2 \langle \Delta v_o \Delta x_o \rangle^2}{\Delta x_\ell^2}. \tag{104}$$

If $x_o$ and $v_o$ are uncorrelated, we can rewrite this expression for $(\Delta x_i)^2_{\min}$ as

$$(\Delta x_i)^2_{\min} = \frac{t_i^2}{t_o^2} t_o^2 \Delta v_o^2 \gamma^2 = \frac{t_i^2}{t_o^2} \Delta x_o^2 (1-\gamma^2). \tag{105}$$

Note that for a harmonic lens, $\delta A = 0$, and

$$(\Delta v_\ell)^2_{\text{bound}} \equiv \frac{(\Delta x_i)^2_{\min}}{t_i^2} = \Delta v_\ell^2 \tag{106}$$

so the refocused cloud size is an unbiased estimator of the collimated temperature.

## B. Gaussian aberrations

A Gaussian potential has the form $V(x,y) = -m\Phi e^{-2(x^2+y^2)/\sigma^2}$, where $\sigma$ is the $1/e^2$ radial waist of the beam. The acceleration in the $x$-direction induced by this potential is

$$a_x(x,y) = -\frac{4\Phi}{\sigma^2} x e^{-2(x^2+y^2)/\sigma^2} \equiv -\omega^2 x e^{-2(x^2+y^2)/\sigma^2} \tag{107}$$

In this section, we assume the initial position and velocity distributions of the ensemble to be 2D Gaussians given by

$$\begin{aligned} W(x,y,v_x,v_y) = {} & \frac{1}{2\pi \Delta x_o \Delta v_{ox}\sqrt{1-\beta_x^2}} \exp\left[-\frac{1}{2(1-\beta_x^2)}\left(\frac{x^2}{\Delta x_o^2} + \frac{v_x^2}{\Delta v_{ox}^2} - 2\frac{\beta_x x v_x}{\Delta x_o \Delta v_{ox}}\right)\right] \\ & \times \frac{1}{2\pi \Delta y_o \Delta v_{oy}\sqrt{1-\beta_y^2}} \exp\left[-\frac{1}{2(1-\beta_y^2)}\left(\frac{y^2}{\Delta y_o^2} + \frac{v_y^2}{\Delta v_{oy}^2} - 2\frac{\beta_y y v_y}{\Delta y_o \Delta v_{oy}}\right)\right] \end{aligned} \tag{108}$$

where

$$\beta_x \equiv \frac{\langle \Delta v_{ox} \Delta x_o \rangle}{\Delta x_o \Delta v_{ox}} \qquad \text{and} \qquad \beta_y \equiv \frac{\langle \Delta v_{oy} \Delta y_o \rangle}{\Delta y_o \Delta v_{oy}} \tag{109}$$

are parameters that characterize the position-velocity correlation in the initial distribution, and we have $|\beta_x| \leq 1$ and $|\beta_y| \leq 1$.

We compute the minimum velocity width $\Delta v_\ell^2$ in the $x$-direction and the collimation lensing time $\delta t_c$ by performing the integrals in Eq. 79 and minimizing with respect to $\delta t$:

$$\Delta v_\ell^2 = \Delta v_{ox}^2 \left( 1 - (1 - \gamma^2 + \beta_x^2 \gamma^2) \frac{(1+8\alpha_x^2)^{3/2}}{(1+4\alpha_x^2)^3} \frac{(1+8\alpha_y^2)^{1/2}}{(1+4\alpha_y^2)} \right) \tag{110}$$

$$\delta t_c = \frac{1}{\omega^2 t_o} \left( 1 - \gamma^2 - \frac{\langle \Delta v_{ox} \Delta x_o \rangle t_o}{\Delta x_\ell^2} \right) \left( \frac{1+8\alpha_x^2}{1+4\alpha_x^2} \right)^{3/2} \left( \frac{1+8\alpha_y^2}{1+4\alpha_y^2} \right)^{1/2} \tag{111}$$

where $\alpha_x^2 \equiv \Delta x_\ell^2/\sigma^2$ and $\alpha_y^2 \equiv \Delta y_\ell^2/\sigma^2$ parameterize the width of the cloud at the lensing plane with respect to the width of the beam.

Similarly, we compute $(\Delta x_i)^2_{\text{min}}$ and $\delta t_{\text{min}}$ by performing the integrals in Eq. 83 and minimizing with respect to $\delta t$, which yields

$$\begin{aligned}(\Delta x_i)^2_{\text{min}} = {} & \Delta x_o^2 + 2 \langle \Delta v_{ox} \Delta x_o \rangle (t_i + t_o) + \Delta v_{ox}^2 (t_i + t_o)^2 \\ & - \Delta x_\ell^2 \left( 1 + \frac{t_i}{t_o} \left( 1 - \gamma^2 - \frac{\langle \Delta v_{ox} \Delta x_o \rangle t_o}{\Delta x_\ell^2} \right) \right)^2 \frac{(1+8\alpha_x^2)^{3/2}}{(1+4\alpha_x^2)^3} \frac{(1+8\alpha_y^2)^{1/2}}{(1+4\alpha_y^2)} \end{aligned} \tag{112}$$

and

$$\delta t_{\text{min}} = \frac{1}{\omega^2} \left( \frac{1}{t_i} + \frac{1}{t_o} \left( 1 - \gamma^2 - \frac{\langle \Delta v_{ox} \Delta x_o \rangle t_o}{\Delta x_\ell^2} \right) \right) \left( \frac{1+8\alpha_x^2}{1+4\alpha_x^2} \right)^{3/2} \left( \frac{1+8\alpha_y^2}{1+4\alpha_y^2} \right)^{1/2} \tag{113}$$

Note that when the size of the cloud at the lens is much less than the size of the beam, $\Delta x_\ell \ll \sigma$ and $\Delta y_\ell \ll \sigma$, then $\alpha_x, \alpha_y \to 0$ and we recover the harmonic case. In addition, the difference between $(\Delta x_i)^2_{\text{min}}/t_i^2$ and $\Delta v_\ell^2$ is the aberration during refocus $\delta A$:

$$\delta A = \frac{\Delta x_\ell^2}{t_i^2} \left( 1 + 2 \frac{t_i}{t_o} \left( 1 - \gamma^2 - \frac{\langle \Delta v_{ox} \Delta x_o \rangle t_o}{\Delta x_\ell^2} \right) \right) \left( 1 - \frac{(1+8\alpha_x^2)^{3/2}}{(1+4\alpha_x^2)^3} \frac{(1+8\alpha_y^2)^{1/2}}{(1+4\alpha_y^2)} \right) \tag{114}$$

Since we have $\left| \langle \Delta v_{ox} \Delta x_o \rangle t_o / \Delta x_\ell^2 \right| \leq (\Delta v_{ox} t_o) \Delta x_o / \Delta x_\ell^2 \approx \gamma \ll 1$, it is clear by inspection that $\delta A > 0$, so $(\Delta v_\ell)_{\text{bound}}$ is an upper bound on the collimated temperature.

### C. High spatial frequency aberrations

In this section, we consider potentials of the form

$$V(x_\ell) = \frac{m\omega^2}{2} x_\ell^2 - m \delta\Phi \sin(k x_\ell + \phi) \tag{115}$$

which induce accelerations of the form

$$a(x_\ell) = -\omega^2 x_\ell + \delta\Phi k \cos(k x_\ell + \phi). \tag{116}$$

We assume that the aberration has a high spatial frequency, so its wavelength $2\pi/k$ is much smaller than any size scale associated with the initial phase space distribution $W(x_o, v_o)$. In addition, we assume that the aberrations are weak compared to the harmonic potential, so

$$\delta\Phi^2 k^2 \ll \omega^4 \Delta x_\ell^2. \tag{117}$$

From Eq. 82, the minimum achievable velocity width is

$$\Delta v_\ell^2 = \frac{\omega^4 \left( \Delta v_o^2 \Delta x_o^2 - \langle \Delta x_o \Delta v_o \rangle^2 \right) + \delta\Phi^2 k^2 \Delta v_o^2 \langle \cos^2(k x_\ell + \phi) \rangle}{\Delta a^2} + \frac{C}{\Delta a^2} \tag{118}$$

where we have used the fact that $x_\ell = x_o + v_o t_o$, and where

$$C = 2\omega^2 \delta\Phi k \left(-\Delta v_o^2 \left\langle \Delta x_o \cos(kx_\ell + \phi)\right\rangle + \left\langle \Delta x_o \Delta v_o\right\rangle \left\langle \Delta v_o \cos(kx_\ell + \phi)\right\rangle\right) - \delta\Phi^2 k^2 \left\langle \Delta v_o \cos(kx_\ell + \phi)\right\rangle^2 . \tag{119}$$

Since the aberrations oscillate rapidly with respect to the initial phase space distribution, $\langle \Delta x_o \cos(kx_\ell + \phi)\rangle = \langle \Delta v_o \cos(kx_\ell + \phi)\rangle = 0$, so $C = 0$, and we have

$$\Delta v_\ell^2 = \frac{\omega^4 \left(\Delta v_o^2 \Delta x_o^2 - \langle \Delta x_o \Delta v_o\rangle^2\right) + \delta\Phi^2 k^2 \Delta v_o^2 \left\langle \cos^2(kx_\ell + \phi)\right\rangle}{\omega^4 \Delta x_\ell^2 + \delta\Phi^2 k^2 \left\langle \cos^2(kx_\ell + \phi)\right\rangle}. \tag{120}$$

Dividing the numerator and denominator by $\omega^4 \Delta x_\ell^2$ and re-writing $\Delta v_\ell^2$ in terms of the small parameter

$$\epsilon \equiv \frac{\delta\Phi^2 k^2}{\omega^4 \Delta x_\ell^2} \left\langle \cos^2(kx_\ell + \phi)\right\rangle \tag{121}$$

we obtain

$$\Delta v_\ell^2 = \frac{1}{1+\epsilon} \left((\Delta v_\ell^H)^2 + \epsilon \, \Delta v_o^2\right) \tag{122}$$

where $\Delta v_\ell^H$ is the minimum velocity width achieved by an ideal harmonic lens. To first order in $\epsilon$, we have

$$\Delta v_\ell^2 \approx (\Delta v_\ell^H)^2 + \epsilon \, \left(\Delta v_o^2 - (\Delta v_\ell^H)^2\right). \tag{123}$$

If $\langle \Delta x_o \Delta v_o\rangle = 0$, we may re-write this expression as

$$\Delta v_\ell^2 \approx (\Delta v_\ell^H)^2 + \epsilon \, \Delta v_o^2 \left(1 - \gamma^2\right). \tag{124}$$

Thus, for high spatial frequency aberrations in the lensing potential with amplitude $\delta\Phi$ and wavelength $2\pi/k$, the heating due to the aberrations scales as $\delta\Phi^2 k^2 (\delta t_c^H)^2$, where $\delta t_c^H$ is the lens duration required to collimate the cloud with an ideal harmonic lens. Note that $\epsilon$ can also be expressed using the expression for $\omega$ for a Gaussian beam from the previous section as

$$\epsilon = \frac{1}{32} (k\sigma)^2 \left(\frac{\delta\Phi}{\Phi}\right)^2 \left(\frac{\sigma}{\Delta x_\ell}\right)^2 \tag{125}$$

where we have taken $\left\langle \cos^2(kx_\ell + \phi)\right\rangle = \frac{1}{2}$. For a Gaussian beam with intensity aberrations, the term $(\delta\Phi/\Phi)$ is the fractional intensity perturbation amplitude at frequency $k$. Aberrations cause significant heating when $\epsilon$ is not negligible compared to $\gamma^2$. For high spatial frequency perturbations ($k\sigma > 1$), the fractional size of the intensity perturbation $(\delta\Phi/\Phi)$ must be made sufficiently small to avoid this source of heating.

### D. Scaling of aberration contributions to cloud size with lens duration

Here we show that in our experiment, the imaged cloud size is the sum in quadrature of the relay image size (i.e. the cloud size produced by a perfect harmonic lens) and an aberration term that scales with the lens application time $\delta t$. We begin by writing the acceleration induced by a general lens potential as $a(x_\ell) = -\omega^2 x_\ell + \delta a(x_\ell)$. Furthermore, we are free to incorporate the linear effect of the aberrations into the definition of $\omega$, so

$$\omega^2 = -\frac{\langle \Delta x_\ell \Delta a\rangle}{\Delta x_\ell^2} \tag{126}$$

and $\langle \Delta x_\ell \Delta \delta a\rangle = 0$.

Combining Eq. 83 and Eq. 84, the imaged cloud size as a function of $\delta t$ is

$$\Delta x_i^2 = \left\langle (\Delta x_o + \Delta v_o(t_o + t_i))^2\right\rangle + 2\left\langle \Delta x_o \Delta a\right\rangle t_i \delta t + 2\left\langle \Delta v_o \Delta a\right\rangle (t_o + t_i) t_i \delta t + \Delta a^2 t_i^2 \delta t^2 \tag{127}$$

Substituting $a = -\omega^2 x_\ell + \delta a$, we have

$$\Delta x_i^2 = (\Delta x_i^H)^2 + \delta X^2 \tag{128}$$

where

$$(\Delta x_i^H)^2 \equiv \left\langle (\Delta x_o + \Delta v_o(t_o+t_i))^2 \right\rangle - 2\left\langle \Delta x_o \Delta x_\ell \right\rangle \omega^2 t_i \delta t - 2\left\langle \Delta v_o \Delta x_\ell \right\rangle \omega^2 (t_o+t_i) t_i \delta t + \Delta x_\ell^2 \omega^4 t_i^2 \delta t^2 \tag{129}$$

is the relay image size, and

$$\delta X^2 \equiv 2\left\langle \Delta x_o \Delta \delta a \right\rangle t_i \delta t + 2\left\langle \Delta v_o \Delta \delta a \right\rangle (t_o+t_i) t_i \delta t + \Delta \delta a^2 t_i^2 \delta t^2 \tag{130}$$

is the contribution from aberrations. Recalling that $x_\ell = x_o + v_o t_o$ and using the fact that $\langle \Delta x_\ell \Delta \delta a \rangle = 0$, we can rewrite $\delta X^2$ as

$$\delta X^2 = -2\left\langle \Delta x_o \Delta \delta a \right\rangle \frac{t_i}{t_o} t_i \delta t + \Delta \delta a^2 t_i^2 \delta t^2. \tag{131}$$

Defining the velocity kick due to the abberations as $\delta v(x_\ell) \equiv \delta a(x_\ell)\delta t$, we have

$$\delta X^2 = -\frac{2}{t_o}\left\langle \Delta x_o \Delta \delta v \right\rangle t_i^2 + \Delta \delta v^2 t_i^2. \tag{132}$$

To establish that the first term in $\delta X^2$ is a small correction, we make three assumptions. First, we assume that the aberrations do not vary significantly with $x_o$ over the region where $W$ has support. That is,

$$\left\langle \left(\frac{\partial \delta v}{\partial x_o}\right)^2 \right\rangle \Delta x_o^2 \ll \Delta \delta v^2. \tag{133}$$

This claim is physically motivated by the fact that $\Delta x_o \approx 50$ $\mu$m; variations in the laser intensity with this length scale diffract out of the beam before it reaches the atoms. Second, we assume that $t_o$ is long enough that

$$\Delta x_o^2 / t_o^2 \lesssim \Delta \delta v^2. \tag{134}$$

Finally, we choose coordinates so that $\langle x_o \rangle = 0$ and assume that $\delta v$ and $x_o$ are uncorrelated at zeroth order in $x_o$, so

$$\left\langle \Delta x_o \Delta \delta v(v_o t_o) \right\rangle = 0. \tag{135}$$

With these assumptions, we can Taylor expand $\delta v(x_o + v_o t_o)$ around $x_o = 0$,

$$\delta v(x_o + v_o t_o) \approx \delta v(v_o t_o) + x_o \frac{\partial \delta v}{\partial x_o} + \cdots \tag{136}$$

and substitute for $\delta v$ in the first term in $\delta X^2$, which yields

$$\frac{1}{t_o}\left\langle \Delta x_o \Delta \delta v \right\rangle = \frac{1}{t_o}\iint x_o \delta v(x_o + v_o t_o) W(x_o, v_o) dx_o dv_o \approx \frac{1}{t_o}\iint x_o \left(\delta v(v_o t_o) + \frac{\partial \delta v}{\partial x_o} x_o\right) W(x_o, v_o) dx_o dv_o. \tag{137}$$

The first term in this integral evaluates to zero by Eq. 135. The remaining term is

$$\frac{1}{t_o}\left\langle \Delta x_o \Delta \delta v \right\rangle = \frac{1}{t_o}\iint x_o^2 \frac{\partial \delta v}{\partial x_o} W(x_o, v_o) dx_o dv_o = \frac{1}{t_o}\left\langle x_o^2 \frac{\partial \delta v}{\partial x_o} \right\rangle. \tag{138}$$

Using the Cauchy-Schwarz inequality, we see that the magnitude of term is less than

$$\frac{1}{t_o}\left\langle \Delta x_o \Delta \delta v \right\rangle \le \frac{1}{t_o}\left(\left\langle x_o^4 \right\rangle \left\langle \left(\frac{\partial \delta v}{\partial x_o}\right)^2 \right\rangle\right)^{1/2} \sim \frac{1}{t_o}\left((\Delta x_o^2)^2 \left\langle \left(\frac{\partial \delta v}{\partial x_o}\right)^2 \right\rangle\right)^{1/2} = \frac{\Delta x_o^2}{t_o}\left\langle \left(\frac{\partial \delta v}{\partial x_o}\right)^2 \right\rangle^{1/2} \tag{139}$$

But by assumption,

$$\left\langle \left(\frac{\partial \delta v}{\partial x_o}\right)^2 \right\rangle \Delta x_o^2 \ll \Delta \delta v^2 \quad \text{and} \quad \Delta x_o^2 / t_o^2 \lesssim \Delta \delta v^2 \tag{140}$$

so

$$\frac{1}{t_o}\left\langle \Delta x_o \Delta \delta v \right\rangle \le \frac{\Delta x_o^2}{t_o}\left\langle \left(\frac{\partial \delta v}{\partial x_o}\right)^2 \right\rangle^{1/2} = \left(\left\langle \left(\frac{\partial \delta v}{\partial x_o}\right)^2 \right\rangle \Delta x_o^2\right)^{1/2} \left(\frac{\Delta x_o^2}{t_o^2}\right)^{1/2} \ll \Delta \delta v^2 \tag{141}$$

and the dominant contribution to $\delta X^2$ comes from the $\langle \delta v^2 \rangle$ term:

$$\delta X^2 \approx \Delta\delta v^2 t_i^2 = \Delta\delta a^2 t_i^2 \delta t^2. \tag{142}$$

The imaged cloud size is therefore

$$\Delta x_i^2 = (\Delta x_i^H)^2 + \Delta\delta a^2 t_i^2 \delta t^2, \tag{143}$$

which is a sum in quadrature of the relay image size and an aberration term that scales with the lens duration $\delta t$.

Since collimating the cloud requires a shorter lens application time than refocusing the cloud, we can correct for the aberration $\delta A$ that occur during refocusing and generate an unbiased estimate of $\Delta v_\ell^2$ by multiplying the aberration contribution by a factor of

$$(\delta t_c/\delta t_{\min})^2 = \frac{(1-\gamma^2)^2}{(\frac{t_o}{t_i}+1-\gamma^2)^2} \tag{144}$$

where aberrations do not change the ratio $\delta t_c/\delta t_{\min}$ significantly for our configuration. Inserting the experimental parameters $t_o = 1.1$ s, $t_i = 1.8$ s, and $\gamma^2 = 0.017$, we find that

$$(\delta t_c/\delta t_{\min})^2 = 0.37. \tag{145}$$

The relay image size is given by

$$\Delta x_i^H = \frac{t_i}{t_o}\sqrt{(1-\gamma^2)}\Delta x_o = 88\ \mu\text{m}. \tag{146}$$

We measure $(\Delta x_i)_{\min} = 110 \pm 30\ \mu$m for the North axis and $120 \pm 40\ \mu$m for the West axis, so $\sqrt{\delta X^2} = 70\ \mu$m for the North axis and 90 $\mu$m for the West axis. Scaling $\delta X^2$ for each axis by $(\delta t_c/\delta t_{\min})^2$, we obtain collimated velocity estimates $(\Delta v_\ell)_{\text{est}} = 55\ \mu$m/s for the North axis and 58 $\mu$m/s for the West axis, which correspond to temperature estimates of 30 pK and 35 pK at collimation.

## IV. POINT SPREAD FUNCTION

As stated in the main text, in order to perform the convolution of the Gaussian atom cloud profile with the PSF, we use a smooth representation of the PSF. We find that a sum of three Gaussians, with parameters fixed as described in the text, provides an accurate representation of the PSF. The choice of the triple Gaussian model is purely phenomenological, and the model's exact functional form is unimportant. For instance, a model consisting of a Gaussian convolved with the sum of two exponential decays can also be used to closely represent the PSF, and the choice of this model vs. the triple Gaussian model does not substantially affect the extracted widths of the lensed clouds.

Explicitly, the triple Gaussian model for the PSF has the form

$$\text{PSF}(x) = \frac{c_1}{w_1\sqrt{2\pi}}e^{-x^2/(2w_1^2)} + \frac{c_2}{w_2\sqrt{2\pi}}e^{-x^2/(2w_2^2)} + \frac{c_3}{w_3\sqrt{2\pi}}e^{-x^2/(2w_3^2)}. \tag{147}$$

Images are fit by the convolution $\phi(x) \otimes \text{PSF}(x)$ of a Gaussian profile $\phi(x) = (\sigma_x\sqrt{2\pi})^{-1}e^{-x^2/(2\sigma_x^2)}$ with the PSF. The parameters $\vec{\alpha} \equiv (c_1, c_2, c_3, w_1, w_2, w_3)$ of the PSF are fixed by fitting $\phi(x) \otimes \text{PSF}(x)$ to a cloud with known, small size $\sigma_x$.

## V. SPONTANEOUS HEATING RATE LIMIT

The dipole lensing results in the main text constrain possible spontaneous heating rates for a free gas of Rb atoms. In particular, many proposed classicalizing modifications to quantum mechanics predict such fundamental heating [3, 4]. Our results therefore restrict the parameter space of these theories. In the following sections, we first outline some similarities between a classical stochastic heating model and the heating that arises from the classicalizing modification to quantum mechanics presented in [3]. We then analyze the effect that this heating would have on the atom refocusing sequence and find that the refocusing data constrain the heating rate for $^{87}$Rb to $20 \pm 30$ pK/s.

### A. Heating from a classicalizing modification to quantum mechanics

In [3] and [5], the authors present a general classicalizing modification to quantum mechanics and show that it leads to fundamental heating. We summarize the relevant results here to motivate the form of the heating rate that we analyze in subsequent sections. A linear modification of the quantum Liouville equation is considered, such that

$$\frac{\partial \rho}{\partial t} = -\frac{i}{\hbar}\left[H, \rho\right] + \mathcal{L}\rho, \tag{148}$$

where $\rho$ is the density matrix and $\mathcal{L}$ is a Lindblad operator corresponding to the classicalizing modification. This causes off-diagonal terms in the density matrix to decay over time, such that the state evolves into a classical mixture. For the form of $\mathcal{L}$ considered in [3], interference effects beyond a critical length scale $\hbar/\sigma_q$ or a critical momentum scale $\hbar/\sigma_s$ decay in a characteristic time $\tau$.

The time evolution of the expectation value of an observable $\hat{A}$ under the classicalizing modification is [5]

$$\partial_t \left\langle \hat{A} \right\rangle = \frac{i}{\hbar}\left\langle [\hat{H}, \hat{A}] \right\rangle + \left\langle \mathcal{L}^\dagger \hat{A} \right\rangle. \tag{149}$$

This corresponds to the Ehrenfest theorem, but with an additional term. For the form of $\mathcal{L}$ considered in [3], the additional term affects the time evolution of expectation values of the position and momentum operators only at second order and above. Specifically, for the free space evolution and harmonic lens of the delta-kick cooling sequence, the time evolution of the relevant operators is [5]

$$\partial_t \left\langle \hat{\mathbf{r}} \right\rangle = \frac{\left\langle \hat{\mathbf{p}} \right\rangle}{m} \tag{150}$$

$$\partial_t \left\langle \hat{\mathbf{p}} \right\rangle = -m\omega^2 \left\langle \hat{\mathbf{r}} \right\rangle \tag{151}$$

$$\partial_t \left\langle \hat{\mathbf{r}}^2 \right\rangle = \frac{1}{m}(\left\langle \hat{\mathbf{p}} \cdot \hat{\mathbf{r}} + \hat{\mathbf{r}} \cdot \hat{\mathbf{p}} \right\rangle) + \frac{\sigma_s^2}{\tau} \tag{152}$$

$$\partial_t \left\langle \hat{\mathbf{p}} \cdot \hat{\mathbf{r}} \right\rangle = \partial_t \left\langle \hat{\mathbf{r}} \cdot \hat{\mathbf{p}} \right\rangle = \frac{1}{m}\left\langle \hat{\mathbf{p}}^2 \right\rangle - m\omega^2 \left\langle \hat{\mathbf{r}}^2 \right\rangle \tag{153}$$

$$\partial_t \left\langle \hat{\mathbf{p}}^2 \right\rangle = -m\omega^2 \left\langle \hat{\mathbf{p}} \cdot \hat{\mathbf{r}} + \hat{\mathbf{r}} \cdot \hat{\mathbf{p}} \right\rangle + \frac{\sigma_q^2}{\tau} \tag{154}$$

The terms with $\omega$ are nonzero only during the lens application time. The classicalizing modification causes deviation from the original equations of motion by introducing an additional diffusion in both momentum and position space, characterized by a constant heating rate $\frac{\sigma_q^2}{2m\tau}$ $(\frac{J}{s})$ and a spreading rate $\frac{\sigma_s^2}{\tau}$ $(\frac{m^2}{s})$.

### B. Analogous classical model: Fokker-Planck equation with a stochastic force

In parallel to the results of Sec. V A, the classical Fokker-Planck model produces unmodified equations of motion for first moments of a phase space distribution, and an additional constant rate of increase in second moments. This model describes the altered evolution of an otherwise deterministic system due to stochastic white noise forces.

We work in terms of the one-dimensional variables $x$ and $v$ for a single particle's parameter space. Under the Fokker-Planck model, a set of generalized stochastic forces $\eta_x$ and $\eta_v$ continuously alter deterministic phase space trajectories via

$$\frac{d}{dt}\begin{bmatrix} x(t) \\ v(t) \end{bmatrix} = \begin{bmatrix} v(t) \\ -\frac{1}{m}\partial_x V \end{bmatrix} + \begin{bmatrix} \eta_x(t) \\ \eta_v(t) \end{bmatrix} \tag{155}$$

The curly bracket notation $\{g(\eta(t))\}$ will be used to define the noise-averaged value of a stochastic variable, where "stochastic variable" is defined as the variable $\eta(t)$ itself or any function g which depends on the stochastic term. The angle bracket notation retains its meaning as an expectation value over the phase space distribution.

As Gaussian white noise terms, the forces $\eta$ have the following properties:

1. The distributions $\eta_x(t)$ and $\eta_v(t)$ at a given time $t$ each have a mean value of zero: $\{\eta_v(t)\} = \{\eta_x(t)\} = 0$.

2. The distribution $\eta_v$ is delta-correlated in time: $\{\eta_v(t_1)\eta_v(t_2)\} = D_v\delta(t_2 - t_1)$.

3. The distribution $\eta_x$ is also delta-correlated: $\{\eta_x(t_1)\eta_x(t_2)\} = D_x\delta(t_2 - t_1)$.

4. The separate distributions are uncorrelated: $\{\eta_v(t_1)\eta_x(t_2)\} = 0$.

Here $D_x$ and $D_v$ are constants characterizing the strengths of the stochastic forces. Due to the stochastic forces, the first moments of a noise-averaged trajectory evolve according to the original equations of motion given by Hamilton's equations, and a modifying term is added to the time evolution of the second moments. Taking first the phase-space ensemble average and next the noise average of Eq. 155 for a harmonic potential, and applying the noise-average properties of $\eta$:

$$\{\partial_t \langle x\rangle\} = \{\langle v\rangle\} \tag{156}$$

$$\{\partial_t \langle v\rangle\} = -\omega^2 \{\langle x\rangle\} \tag{157}$$

$$\left\{\partial_t \left\langle x^2\right\rangle\right\} = 2\{\langle x\cdot v\rangle\} + D_x \tag{158}$$

$$\{\partial_t \langle x\cdot v\rangle\} = \left\{\left\langle v^2\right\rangle\right\} - \omega^2\left\{\left\langle x^2\right\rangle\right\} \tag{159}$$

$$\left\{\partial_t \left\langle v^2\right\rangle\right\} = -2\omega^2\{\langle x\cdot v\rangle\} + D_v \tag{160}$$

Again, the terms with $\omega$ are only nonzero during the lens application time. Eqs. 150 through 154 (for the effect of the Lindblad operator), and Eqs. 156 through 160 (for the classical Fokker-Planck model model of diffusion) therefore form an analogous set of differential equations for moments up to second order of a distribution. The connection is made concrete by setting $D_x = \frac{1}{3}\frac{\sigma_s^2}{\tau}$, and $D_v = \frac{1}{3}\frac{\sigma_q^2}{m^2\tau}$ (the factor of 1/3 arises because we are now considering a 1D problem).

An expression can now be derived for final width of the cloud in terms of $D_v$ and $D_x$ by considering evolution of classical trajectories. Given a particular initial value of both $\Delta x_o$ and $\Delta v_o$, we can compare the modeled minimized final width $(\Delta x_i)_{\min}$ under a perfect harmonic lens to the measured value. If the error between the two values is ascribed fully to the modifications introduced by stochastic diffusive terms, then a maximum heating rate is set.

### C. Stochastic modifications of the trajectories

Terms that couple to $\eta_v$ and $\eta_x$ will be expressed in terms of their noise averages. The total change in the trajectory from its deterministic $(x(t), v(t))$ at a time $t$ due to $\eta_v$ is labeled $(\delta x_{\eta_v}(t), \delta v_{\eta_v}(t))$, and the change due to $\eta_x$ is $\delta x_{\eta_x}(t)$. Due to the form of Hamilton's equations of motion, $\eta_x$ does not directly couple to the variable $v(t)$. The changes are given in integral form by

$$\delta v_{\eta_v}(t_1, t_2) = \int_{t_1}^{t_2} \eta_v(t')dt' \tag{161}$$

$$\delta x_{\eta_v}(t_1, t_2) = \int_{t_1}^{t_2}\int_{t_1}^{t'} \eta_v(t'')dt''dt' \tag{162}$$

$$\delta x_{\eta_x}(t_1, t_2) = \int_{t_1}^{t_2} \eta_x(t')dt' \tag{163}$$

Using these definitions, the results of Table I follow from the fact that the stochastic force is independent of phase space trajectory. The results of Table II can be shown from repeated integration of Eq. 155. Table II lists results for

TABLE I. Stochastic variable correlations with initial distribution

| | |
|---|---|
| $\left\{\left\langle \delta x_{\eta_{v,x}}(t_1,t_2)x_o\right\rangle\right\} = 0$ | $\{\langle \delta v_{\eta_v}(t_1,t_2)x_o\rangle\} = 0$ |
| $\left\{\left\langle \delta x_{\eta_{v,x}}(t_1,t_2)v_o\right\rangle\right\} = 0$ | $\{\langle \delta v_{\eta_v}(t_1,t_2)v_o\rangle\} = 0$ |

TABLE II. Noise averages of stochastic variable correlations

| | |
|---|---|
| $\{\langle \delta v_{\eta_v}(t_1,t_2)\delta v_{\eta_v}(t_1,t_2)\rangle\} = D_v(t_2-t_1)$ | $\{\langle \delta x_{\eta_x}(t_1,t_2)\delta x_{\eta_x}(t_1,t_2)\rangle\} = D_x(t_2-t_1)$ |
| $\{\langle \delta x_{\eta_v}(t_1,t_2)\delta x_{\eta_v}(t_1,t_2)\rangle\} = \frac{1}{3}D_v(t_2-t_1)^3$ | $\{\langle \delta v_{\eta_v}(t_1,t_2)\delta x_{\eta_v}(t_1,t_2)\rangle\} = \frac{1}{2}D_v(t_2-t_1)^2$ |

fully overlapping time intervals; for nonoverlapping time intervals, the noise-average product of all stochastic terms in the table is zero.

### D. Delta-kick sequence with stochastic modification

In the following sections, we assume $\langle v_o x_o\rangle = 0$ and that the lens provides a perfect harmonic potential.

#### 1. Object to lens

Directly before the lens ($\ell^-$) and immediately after ($\ell^+$), the noise average position and velocity of a trajectory in phase space are

$$x_{\ell^-} = x_{\ell^+} = x_o + v_o t_o + \delta x_{\eta_v}(0, t_o) + \delta x_{\eta_x}(0, t_o) \tag{164}$$
$$v_{\ell^-} = v_o + \delta v_{\eta_v}(0, t_o) \tag{165}$$
$$v_{\ell^+} = v_o + \delta v_{\eta_v}(0, t_o) - \omega^2 \delta t\, x_{\ell^-} \tag{166}$$

It is assumed that the cooling rate during the lens application is much larger than the heating rate due to diffusion, $\langle v_{\ell^+}^2\rangle - \langle v_{\ell^-}^2\rangle \gg D_v \delta t$, so that the effect of the stochastic modification can be neglected during the time that the atom spends in the harmonic potential. The noise-averaged and ensemble-averaged position and velocity variance after the lens become

$$\left\{\langle \Delta x_{\ell^+}^2\rangle\right\} = \Delta x_o^2 + \Delta v_o^2 t_o^2 + \tfrac{D_v t_o^3}{3} + D_x t_o \tag{167}$$
$$\left\{\langle \Delta v_{\ell^+}^2\rangle\right\} = \Delta v_o^2 + D_v t_o - 2\omega^2 \delta t \left(\Delta v_o^2 t_o + \tfrac{D_v t_o^2}{2}\right) + \omega^4 \delta t^2 \left(\Delta v_o^2 t_o^2 + \Delta x_o^2 + \tfrac{D_v t_o^3}{3} + D_x t_o\right) \tag{168}$$

The results from Table I and Table II have been applied to eliminate or reduce relevant terms.

#### 2. Lens to image

The single-particle position and velocities at the image are

$$v_i = v_{\ell^+} + \delta v_{\eta_v}(t_o, t_o + t_i) \tag{169}$$
$$x_i = t_i v_{\ell^+} + x_{\ell^+} + \delta x_{\eta_v}(t_o, t_o + t_i) + \delta x_{\eta_x}(t_o, t_o + t_i) \tag{170}$$

After neglecting terms with an average value of zero, the noise-averaged, ensemble-averaged position variance at the image takes the form

$$\left\{\langle \Delta x_i^2\rangle\right\} = t_i^2 \left\{\langle \Delta v_{\ell^+}^2\rangle\right\} + \left\{\langle \Delta x_{\ell^+}^2\rangle\right\} + 2t_i \left\{\langle \Delta x_{\ell^+} \Delta v_{\ell^+}\rangle\right\} + \tfrac{D_v t_i^3}{3} + D_x t_i \tag{171}$$

Next, the expressions from Eqs. 167 and 168 are substituted into 171. The cross-correlation term between position and velocity directly after the lens takes the form

$$\left\{\langle \Delta x_{\ell^+} \Delta v_{\ell^+}\rangle\right\} = \Delta v_o^2 t_o + \frac{D_v t_o^2}{2} - \omega^2 \delta t \left(\Delta v_o^2 t_o^2 + \Delta x_o^2 + \tfrac{D_v t_o^3}{3} + D_x t_o\right). \tag{172}$$

#### 3. Constraining the heating rate with refocusing data

Next, we assume that in an experiment, the lens application time will be chosen to minimize the final cloud width. This time is found symbolically as the solution to

$$\frac{\partial \left\{\langle \Delta x_i^2\rangle\right\}}{\partial(\delta t)} = 0. \tag{173}$$

In an ideal deterministic case with an uncorrelated position-velocity distribution, the cloud size at the lens is $\Delta x_\ell^2 = \Delta x_o^2 + t_o^2 \Delta v_o^2$, and the minimum cloud width after refocusing is given by

$$(\Delta x_i)_{\min} = \frac{t_i^2 \Delta v_o^2 \Delta x_o^2}{\Delta x_\ell^2} \tag{174}$$

The minimized cloud size at the image plane using the expression for $\delta t$ from Eqn. 173 becomes

$$(\Delta x_i)_{\min} = \frac{t_i^2 \Delta v_o^2 \Delta x_o^2 + aD_x + bD_v + cD_xD_v + dD_x^2 + eD_v^2}{\Delta x_\ell^2 + \frac{D_v t_o^3}{3} + D_x t_o} \tag{175}$$

where

$$\begin{aligned} a &= t_i \Delta x_\ell^2 \left(1 + \frac{t_i}{t_o}(1-\gamma^2)\right) \\ b &= \frac{1}{3} t_i^2 t_o \Delta x_\ell^2 \left(1 + \frac{t_i}{t_o} + 2\gamma^2\right) \\ c &= \frac{1}{3} t_i t_o (t_i^2 + 3t_i t_o + t_o^2) \\ d &= t_i t_o \\ e &= \frac{1}{36} t_i^2 t_o^3 (4t_i + 3t_o) \end{aligned} \tag{176}$$

Given experimentally measured distributions $\Delta x_o^2$, and $\Delta v_o^2$, and parameters $t_o$ and $t_i$, there is in general a discrepancy between the ideal $\Delta x_i^2$ given in Eq. 174 for a lens application time that minimizes the width, and the experimentally measured final cloud width. Here we consider spontaneous heating attributed solely to $D_v$ and set $D_x = 0$ (this is the case for spontaneous localization theories) [3]. In this case, the larger solution to the quadratic equation defined by Eq. 175 for $D_v$ is given by $D_v = \frac{-B+\sqrt{B^2-4AC}}{2A}$, where

$$\begin{aligned} A &= t_i^2 t_o^3 (4t_i + 3t_o) \\ B &= 12\left(t_i^3 \Delta x_\ell^2 \left(1 + \frac{t_o}{t_i}(1+2\gamma^2)\right) - t_o^3 (\Delta x_i)_{\min}^2\right) \\ C &= 36(t_i^2 \Delta v_o^2 \Delta x_o^2 - (\Delta x_i)_{\min}^2 \Delta x_\ell^2) \end{aligned} \tag{177}$$

In the present experiment, the evolution times were $t_o = 1.1$s and $t_i = 1.8$ s. The initial cloud effective temperature was $1.6 \pm 0.1$ nK (corresponding to $\Delta v_o = 0.39$ mm/sec). The initial cloud width is $\Delta x_o = 56$ $\mu$m and the final refocused cloud width is $(\Delta x_i)_{\min} = 120 \pm 40$ $\mu$m. Based on these parameters, we set a bound on the spontaneous heating rate of $mD_v/k_{\rm B} = 20 \pm 30$ pK/s. As discussed in [3], this limit on a fundamental heating rate can be compared to other experiments that test quantum mechanics in the macroscopic regime using the relation $D_v = \frac{1}{3}\frac{\sigma_q^2}{m^2\tau}$.

---


[1] E. Giese, W. Zeller, S. Kleinert, M. Meister, V. Tamma, A. Roura, and W. P. Schleich, "The interface of gravity and quantum mechanics illuminated by Wigner phase space," (2014), arXiv:arXiv:1402.0963v1.

[2] B. Dubetsky and M. Kasevich, Physical Review A, **74**, 023615 (2006), ISSN 1050-2947.

[3] S. Nimmrichter and K. Hornberger, Physical Review Letters, **110**, 160403 (2013), ISSN 0031-9007, arXiv:arXiv:1205.3447v2.

[4] A. Bassi, K. Lochan, S. Satin, T. Singh, and H. Ulbricht, Reviews of Modern Physics, **85**, 471 (2013), ISSN 0034-6861.

[5] S. Nimmrichter, *Macroscopic Matter-wave Interferometry*, Ph.D. thesis (2013).

[6] Such a modification causes off-diagonal terms in the density matrix to decay over a characteristic time, causing the matrix to evolve toward that of a classical mixed state with loss of phase coherence between eigenstates and therefore a loss of quantum interference effects beyond characteristic length and momentum scales.

[7] S. M. Dickerson, J. M. Hogan, A. Sugarbaker, D. M. S. Johnson, and M. A. Kasevich, Physical Review Letters, **111**, 083001 (2013), ISSN 0031-9007, arXiv:arXiv:1305.1700v1.
